# Supplementary material for: Signatures of discrete time-crystallinity in transport through an open Fermionic chain
Source: arXiv:2107.04214 ancillary file (2022-05-14)
Supplement: Supplementary file 1 [file SI_Transport_signatures_of_Dissipative_time_crystals.pdf]

# Supplementary Information: Signatures of discrete time-crystallinity in transport through an open Fermionic chain

Subhajit Sarkar*
*Department of Chemistry, Ben-Gurion University of the Negev, Beer Sheva, 84105, Israel and School of Electrical and Computer Engineering, Ben-Gurion University of the Negev, Beer Sheva, 84105, Israel*

Yonatan Dubi†
*Department of Chemistry, Ben-Gurion University of the Negev, Beer Sheva, 84105, Israel and Ilse Katz Center for Nanoscale Science and Technology, Ben-Gurion University of the Negev, Beer Sheva, 84105, Israel*

(Dated: May 14, 2022)

## CONTENTS

SUPPLEMENTARY NOTE 1. Generalization of the Floquet dynamical symmetry in presence of dynamical symmetry breaking jump operators 1

SUPPLEMENTARY NOTE 2. Weak local FDS as an emergent property near the FSS 5

SUPPLEMENTARY NOTE 3. Notion of weak-Floquet dynamical symmetry 6

SUPPLEMENTARY NOTE 4. System size N=5 6

SUPPLEMENTARY NOTE 5. Dephasing rate dependence of sub-harmonic synchronization 7

SUPPLEMENTARY NOTE 6. Spin-current 8

References 8

## SUPPLEMENTARY NOTE 1. GENERALIZATION OF THE FLOQUET DYNAMICAL SYMMETRY IN PRESENCE OF DYNAMICAL SYMMETRY BREAKING JUMP OPERATORS

For time periodic Liouvillian $\mathcal{L}(t+T) = \mathcal{L}(t)$ the time evolution operator, a time-dependent map, is defined as,

$$\mathcal{U}(t) = \mathcal{T}\left[\exp\left(\int_0^t \mathcal{L}(t)\ dt'\right)\right], \tag{S1}$$

where $\mathcal{T}$ denotes the time time-ordering [1]. The one period time evolution operator is called the Floquet map and is defined as,

$$\mathcal{U}_F = \mathcal{U}(T) = \mathcal{T}\left[\exp\left(\int_0^T \mathcal{L}(t')\ dt'\right)\right], \tag{S2}$$

where the Liouvillian is given by the standard Markovian Floquet-Lindblad equation [2–5],

$$\frac{d\rho}{dt} = \mathcal{L}(\rho) = -i[H(t),\rho] + \sum_\mu \left(V_\mu \rho V_\mu^\dagger - \frac{1}{2}\{V_\mu^\dagger V_\mu, \rho\}\right), \tag{S3}$$

with the assignment of $\hbar = 1$, the unit of $H(t)$ is expressed in energy and the unit of time (and therefore the period $T$) is expressed in the unit of energy such that $\mathcal{L}(t')\ dt'$ is a dimensionless quantity. The Floquet-Lindblad

* subhajit@post.bgu.ac.il
† jdubi@bgu.ac.il

equation describes trace-preserving non-unitary dynamics for the density matrix $\rho$ for a system having time-periodic Hamiltonian $H(t+T) = H(t)$ describing the unitary part of the evolution, and $V_\mu$'s are the Lindblad operators representing the dissipation [2–5].

An operator $A(t) = \mathcal{U}(t)A\mathcal{U}^{-1}(t)$ represents a Floquet Dynamical Symmetry (FDS) operator if the following FDS conditions are satisfied [6],

$$\begin{aligned} A(T) = \mathcal{U}_F A \mathcal{U}_F^{-1} = e^{-i\lambda T} A, \\ [V_\mu, A(t)] = \left[V_\mu^\dagger, A(t)\right] = 0 \;\forall\; t, \mu. \end{aligned} \tag{S4}$$

The notion of FDS utilizes the existence of a dark state space where the coherence are preserved and exhibited in an oscillatory behavior of the FDS operator $A(t)$.

We aim to generalize the notion of the FDS by illuminating the dark state space, therefore, aiding the measurement of the preserved coherence weakly enough. To this end, we first set the notations by re-deriving the eigenvalue equation for $\mathcal{U}_F$ in absence any system-lead coupling that illuminates the dark-state space.

We can define left and right super-operators $\hat{O}_L$ and $\hat{O}_R$, respectively, such that $\hat{O}_L|\rho_L\rangle\rangle \to O(\rho)$ and $\hat{O}_R|\rho_R\rangle\rangle \to (\rho)O^\dagger$, where $O$ is the "regular operator" in Fock space having the same dimensions as that of the density matrix (DM) $\rho$, say $N \times N$, and $|\rho_{L,R}\rangle\rangle$ is vectorized DM of dimension $N^2 \times 1$, and there exists a mapping $|\rho_R\rangle\rangle \to \rho$ and $|\rho_L\rangle\rangle \to \rho^\dagger$. $O\rho$ represents matrix multiplication in the regular operator space and the symbol $\to$ denotes the mapping . In the super-operator notation in Fock-Liouville space the orthogonality of two arbitrary density matrices are denoted as $\langle\langle\rho_j|\rho_k\rangle\rangle = Tr[\rho_j^\dagger \rho_j] = \delta_{j,k}$, following the notation of [7]. In the super-operator notation FDS implies, $\hat{\mathcal{U}}_F \hat{A}_L = e^{-i\lambda T}\hat{A}_L\hat{\mathcal{U}}_F$, and $\hat{\mathcal{U}}_F \hat{A}_R = e^{i\lambda T}\hat{A}_R\hat{\mathcal{U}}_F$, where $\hat{\mathcal{U}}_F$ is a super-operator corresponding to the one-period Floquet propagator. The coherence defined as $\rho_{mn} = A^m \rho_{FSS}(A^\dagger)^n$ can be written in the super-operator notation as $|\rho_{mn}\rangle\rangle = \hat{A}_L^m \hat{A}_R^n |\rho_{FSS}\rangle\rangle$, where $\rho_{FSS}$ represents the Floquet steady state (FSS), and

$$\begin{aligned} \hat{\mathcal{U}}_F|\rho_{mn}\rangle\rangle &= \hat{\mathcal{U}}_F \hat{A}_L^m \hat{A}_R^n |\rho_{FSS}\rangle\rangle \\ &= e^{-im\lambda T}\hat{A}_L^m \hat{\mathcal{U}}_F \hat{A}_R^n |\rho_{FSS}\rangle\rangle \\ &= e^{-i(m-n)\lambda T}\hat{A}_L^m \hat{A}_R^n |\rho_{FSS}\rangle\rangle \\ &= e^{-i(m-n)\lambda T}|\rho_{mn}\rangle\rangle. \end{aligned} \tag{S5}$$

Then in the "regular operator" notation the above eigen-value equation reads as $\mathcal{U}_F(\rho_{mn}) = e^{-i(m-n)\lambda T}(\rho_{mn})$, with $m = n$ being the Floquet steady state satisfying $\mathcal{U}_F(\rho_{FSS}) = (\rho_{FSS})$. Without the loss of generality one can assume $m - n = -1$, $\forall\ m$, such that $\mathcal{U}_F(\rho_{m,1}) = e^{i\lambda T}(\rho_{m,1})$. These eigen-value equations define the discrete time crystal (DTC) eigen-values as $(\mathcal{E}_{TC})^N = e^{iN\lambda T} = 1$, and the FSS eigen-value as $\mathcal{E}_{FSS} = 1$.

The equation of motion in the Lindblad form for any operator $X(t)$ [as well as the FDS operator $A(t)$] is given by,

$$\frac{dX}{dt} = i[\mathcal{H}(t), X] + \frac{1}{2}\sum_\mu \left(V_\mu^\dagger\left[X, V_\mu\right] + \left[V_\mu^\dagger, X\right]V_\mu\right), \tag{S6}$$

(notice $\hbar = 1$) where the periodic Hamiltonian $\mathcal{H}(t)$ is given by Eq. (4). The index $\mu$ runs over, dephasing, left-lead and right-lead; see Eq. (5) and preceding notations for details. We notice that, for our specific case of Eq. (4) the FDS operator is $S^+ = \sum_{j=1}^N S_j^+$, the total spin raising operator, which we prove below.

Considering the equal-time commutation relation the equation of motion for the total spin raising operator $S^+ = \sum_{j=1}^N S_j^+$ become,

$$\frac{dS^+}{dt} = i[H(t), S^+] + \frac{1}{2}\sum_\mu \left(V_\mu^\dagger\left[S^+, V_\mu\right] + \left[V_\mu^\dagger, S^+\right]V_\mu\right). \tag{S7}$$

Then the following commutation relations hold (due to the underlying SU(2) symmetry),

$$\begin{aligned} \left[\mathcal{H}_0, S^+\right] = 0 \\ \left[\mathcal{H}_0, S^z\right] = 0, \end{aligned} \tag{S8}$$

where the last of the above equation signifies *the $z-$ component of the total spin and the total spin-raising operator are conserved in absence of driving*. Furthermore, $S^+$ is a dark state operator with respect to the on-site dephasing. Given the above commutation relations it is easy to show,

$$\frac{dS^+}{dt} = i[H(t), S^+] - \gamma_L S_1^+ - \gamma_R S_N^+. \tag{S9}$$

One can find a Floquet micro-motion operator [5, 8], $P(t) = e^{i\omega t(NI - \sum_j S^z_j)} = \prod_{\otimes j} e^{i\omega t(I - S^z_j)}$ with $P(t) = P(t+T)$ acting on the site basis, which will transform $H(t)$ into the Floquet basis (rotating frame) where $H(t)$ is equivalent to a (stroboscopic) Floquet Hamiltonian under static magnetic field $\mathbf{h} = (B, 0, \omega)$, viz.,

$$\mathcal{H}_F = P(t)^\dagger \left[H(t) - \partial_t\right] P(t) = \mathcal{H}_0 + \mathbf{h}\cdot\mathbf{S}, \tag{S10}$$

where $|\mathbf{h}| = \sqrt{B^2+\omega^2}$. At this stage we consider that at each site the applied field exhibit the same $(B_x, B_y)$ and $\omega$. This makes $|\mathbf{h}| = \sqrt{B^2+\omega^2}$ the same at each site. It would be interesting to consider the effect of disorder in $(B_x, B_y)$ and $\omega$. Also note that $P^\dagger(t) S^z P(t) = S^z_{|\mathbf{h}|} = S^z$. Defining the total spin raising operator in the Floquet basis as $S^+_{|\mathbf{h}|} = P^\dagger(t) S^+ P(t)$ $(= S^+ e^{i\omega t})$, we can find the equation for the $S^+_{|\mathbf{h}|}$ as,

$$\begin{aligned}
\frac{dS^+_{|\mathbf{h}|}}{dt} &= \dot{P}^\dagger(t) S^+ P(t) + P^\dagger(t)\frac{dS^+}{dt}P(t) + P^\dagger(t) S^+ \dot{P}(t) \\
&= i\omega\left[S^z, S^+_{|\mathbf{h}|}\right] + P^\dagger(t)\frac{dS^+}{dt}P(t) \\
&= i\omega\left[S^z, S^+_{|\mathbf{h}|}\right] + P^\dagger(t)\left[H_{ext}(t), S^+\right]P(t) - \gamma_L S^+_{1,|\mathbf{h}|} - \gamma_R S^+_{N,|\mathbf{h}|} \\
&= i\left[\mathbf{h}\cdot\mathbf{S}, S^+_{|\mathbf{h}|}\right] - \gamma_L S^+_{1,|\mathbf{h}|} - \gamma_R S^+_{N,|\mathbf{h}|} \;\; (\mathbf{h}\cdot\mathbf{S} \text{ an effective Zeeman term}) \\
&= i|\mathbf{h}| S^+_{|\mathbf{h}|} - \gamma_L S^+_{1,|\mathbf{h}|} - \gamma_R S^+_{N,|\mathbf{h}|}
\end{aligned} \tag{S11}$$

where noticing that $S^+_{|\mathbf{h}|} = S^+ e^{i\omega t}$, we can evaluate $\left[\mathbf{h}\cdot\mathbf{S}, S^+_{|\mathbf{h}|}\right] = \left[|\mathbf{h}| S^z_{|\mathbf{h}|}, S^+_{|\mathbf{h}|}\right] = i|\mathbf{h}| S^+_{|\mathbf{h}|}$, where the axis of quantization is now rotated along the direction of $\mathbf{h}$. Notice that using $S^+_{|\mathbf{h}|} = \sum_j S^+_{j,|\mathbf{h}|}$ we can rewrite (S11),

$$\sum_j \frac{dS^+_{j,|\mathbf{h}|}}{dt} = \sum_j \left(i|\mathbf{h}| - \gamma_L \delta_{j,1} - \gamma_R \delta_{j,N}\right) S^+_{j,|\mathbf{h}|}, \tag{S12}$$

where the summation is over site index $j$ and we have assumed the effective field $\mathbf{h}$ is the same for each site (i.e., homogeneous) without the loss of the generality. Since the spin operators act locally on each lattice site, this allows us to solve (S12) for each site, viz., for sites 1 & $N$ we have $\frac{dS^+_{1(N),|\mathbf{h}|}}{dt} = \left(i|\mathbf{h}| - \gamma_{L(R)}\right) S^+_{1(N),|\mathbf{h}|}$, and for the rest of the sites, $\frac{dS^+_{j,|\mathbf{h}|}}{dt} = i|\mathbf{h}| S^+_{j,|\mathbf{h}|}$. Therefore, at each site the solutions of (S12) over one period are given by,

$$\begin{aligned}
\hat{S}^+_{1(N),|\mathbf{h}|}(T) &= \hat{\mathcal{U}}_F \hat{S}^+_{1(N),|\mathbf{h}|} \hat{\mathcal{U}}_F^{-1} = e^{i|\mathbf{h}|T} e^{-\gamma_{L(R)}T} \hat{S}^+_{1(N),|\mathbf{h}|} \\
\hat{S}^+_{j,|\mathbf{h}|}(T) &= \hat{\mathcal{U}}_F \hat{S}^+_{j,|\mathbf{h}|} \hat{\mathcal{U}}_F^{-1} = e^{i|\mathbf{h}|T} S^+_{j,|\mathbf{h}|} \;\; \forall\, j \neq 1 \text{ and } N,
\end{aligned} \tag{S13}$$

respectively in the super-operator notation. This is expected from the fact that only at both ends of the Lattice the leads are connected. Once we remove the leads the above solutions reduce to the conventional FDS for each site. However, (S13) may not be an exact relation at the operator level, rather it emerges near the FSS, see SUPPLEMENTARY NOTE 2 for further clarification.

Furthermore, equation (S12) can be considered as an equation of motion for $S^+_{|\mathbf{h}|}$ generated by a Floquet Lindbladian $\mathcal{L}_F$ whose coherent part, $i\left[(\cdot), \sum_j S^+_{j,|\mathbf{h}|}\right]$, is generated by a Floquet Hamiltonian $\mathcal{H}_F = \mathbf{h}\cdot\sum_j \mathbf{S}_j$, a Zeeman term under an effective homogeneous (the same at each lattice site) and static magnetic field $\mathbf{h}$. Therefore, from now on we work in the Floquet basis (in the rotated frame). Under these circumstances we can define a local operator $S^+_{loc,|\mathbf{h}|} = S^+_{1,|\mathbf{h}|} + S^+_{N,|\mathbf{h}|}$ which can project the full Hilbert-space of the system to the sub-space of the decaying coherent states. This is a local operator because in the site basis it is diagonal, viz., $S^+_{loc,|\mathbf{h}|} = (\underbrace{[S^+_{1,|\mathbf{h}|} \otimes I_2 \otimes \cdots \otimes I_N]}_{\text{block 1}} + \underbrace{[I_1 \otimes I_2 \otimes \cdots \otimes S^+_{N,|\mathbf{h}|}]}_{\text{block 2}})$ with no cross-term (that can lead to possible non-locality) exists between block 1 and block 2. We then consider $\gamma_L = \gamma_R = \gamma$, i.e., the coupling between system with the left electrode is the same as that between the right electrodes. The local super-operator $\hat{S}^+_{loc,|\mathbf{h}|}$ further satisfies $\hat{\mathcal{U}}_F \hat{S}^+_{loc,|\mathbf{h}|} \hat{\mathcal{U}}_F^{-1} = e^{i|\mathbf{h}|T} e^{-\gamma T} \hat{S}^+_{loc,|\mathbf{h}|}$, which in the regular operator notation is given by, $\mathcal{U}_F(S^+_{loc,|\mathbf{h}|}\rho) = S^+_{loc,|\mathbf{h}|}\mathcal{U}_F(\rho)$, and the ad-joint one is given by, $\mathcal{U}_F(\rho S^-_{loc,|\mathbf{h}|}\rho) = \mathcal{U}_F(\rho) S^-_{loc,|\mathbf{h}|}$ for any density matrix $\rho$ satisfying (S3). Thus, it is easy to show that $S^+_{loc,|\mathbf{h}|}$ satisfies the following relation,

$$(\mathcal{U}_F)^p S^+_{loc,|\mathbf{h}|} = e^{ip|\mathbf{h}|T} e^{-p\gamma T} S^+_{loc,|\mathbf{h}|} (\mathcal{U}_F)^p = e^{ip|\mathbf{h}|T(1+i\gamma/|\mathbf{h}|)} S^+_{loc,|\mathbf{h}|} (\mathcal{U}_F)^p, \tag{S14}$$

after $p$ driving periods. Defining, in the super-operator notation,

$$|\rho_{mn}\rangle\rangle = (\hat{S}^{+}_{loc,|\mathbf{h}|})^{m}_{L}(\hat{S}^{-}_{loc,|\mathbf{h}|})^{n}_{R}|\rho_{\mathrm{FSS}}\rangle\rangle,\ m,n \text{ are positive integers,} \tag{S15}$$

for the vectorized Floquet steady state density matrix $|\rho_{\mathrm{FSS}}\rangle\rangle$, and considering $\gamma_L = \gamma_R = \gamma$ it is easy to find that,

$$\hat{\mathcal{U}}_F|\rho_{mn}\rangle\rangle = e^{i(m-n)|\mathbf{h}|T}e^{-(m+n)\gamma T}|\rho_{mn}\rangle\rangle. \tag{S16}$$

In the normal operator notation the above equation is expressed as,

$$\begin{aligned}\mathcal{U}_F\left((S^{+}_{loc,|\mathbf{h}|})^m\rho_{\mathrm{FSS}}(S^{-}_{loc,|\mathbf{h}|})^n\right) &= e^{im|\mathbf{h}|T}e^{-m\gamma T}\mathcal{U}_F\left(\rho_{\mathrm{FSS}}(S^{-}_{loc,|\mathbf{h}|})^n\right)\\ &= e^{i(m-n)|\mathbf{h}|T}e^{-(m+n)\gamma T}(S^{+}_{loc,|\mathbf{h}|})^m\underbrace{[\mathcal{U}_F(\rho_{\mathrm{FSS}})]}_{\rho_{\mathrm{FSS}}}(S^{-}_{loc,|\mathbf{h}|})^n\end{aligned} \tag{S17}$$

for a Floquet steady state $\rho_{\mathrm{FSS}}$. Since $S^{+}_{loc,|\mathbf{h}|}$ does not commute with the Lindblad jump operators corresponding to the system-lead couplings, viz, $V_{L(R),\sigma}$, equation (S17) is the Floquet analogue of the weak dynamical condition for open-systems [9].

Due to decay via the external leads we have one and only one non decaying unique Floquet steady state corresponding to $m = n = 0$, i.e., $|\rho_{00}\rangle\rangle = |\rho_{FSS}\rangle\rangle$. For $m = n$ all the rest of the states are decaying states. For $m \neq n$ $|\rho_{mn}\rangle\rangle$ are the coherent states that has an exponentially decaying envelop.

Therefore, some of the coherent states $|\rho_{mn}\rangle\rangle$ are decaying coherence responsible for the amplitude decay of the DTC, and there are others which are non-decaying, and altogether they form a set of basis states in the super-operator space in which $\mathcal{U}_F$ and $\mathcal{L}_F$ live. However, a mixing between the decaying and non-decaying coherent states lead to an over-all decaying DTC which we call, depending on the magnitude of the system-lead coupling, a meta-stable DTC. It is worthwhile to point out that Ref. [10] havs pointed out that a meta-stable DTC due to deviation from the dynamical symmetry is an open question which may lead to a possibility of dissipative phase transition.

Let us now prove $\langle\langle\rho_{pq}|\rho_{mn}\rangle\rangle \approx \delta_{p,m}\delta_{q,n}$. First we notice that in the regular notation the eigen-matrix $(\rho_{mn})^{\dagger} = \rho_{nm}$. We have $|\langle\langle\rho_{pq}|\hat{\mathcal{U}}_F|\rho_{mn}\rangle\rangle| = e^{-(m+n)\gamma T}|\langle\langle\rho_{pq}|\rho_{mn}\rangle\rangle|$ and similarly $|\langle\langle\rho_{mn}|\hat{\mathcal{U}}_F|\rho_{pq}\rangle\rangle| = e^{-(p+q)\gamma T}|\langle\langle\rho_{mn}|\rho_{pq}\rangle\rangle|$. Given $|\langle\langle\rho_{pq}|\hat{\mathcal{U}}_F|\rho_{mn}\rangle\rangle| = |\langle\langle\rho_{mn}|\hat{\mathcal{U}}_F|\rho_{pq}\rangle\rangle|$ and $|\langle\langle\rho_{pq}|\rho_{mn}\rangle\rangle| = |\langle\langle\rho_{mn}|\rho_{pq}\rangle\rangle|$ one can recognize $p = m$ and $q = n$ must satisfy otherwise the overlap $|\langle\langle\rho_{pq}|\rho_{mn}\rangle\rangle|$ decays, therefore, the ortho-normality of $|\rho_{mn}\rangle\rangle$ holds approximately. A similar ortho-normality has been shown in Ref. [11] for the Lindbladian $\mathcal{L}$. Such an ortho-normality condition for the coherent states along with their spatial transnational invariance are the necessary and sufficient conditions for the space-time synchronized oscillation of $\langle S_{j,|\mathbf{h}|}(t)\rangle$ as explained in Ref. [11].

Finally a DTC density matrix is given by,

$$\begin{aligned}|\rho_{DTC}\rangle\rangle &= \sum_{m,n} c_{m,n}|\rho_{mn}\rangle\rangle = |\rho_{FSS}\rangle\rangle + |\rho_{coh}\rangle\rangle,\\ &= |\rho_{FSS}\rangle\rangle + \sum_{\substack{m,n\\ m,n\neq 0}} c_{m,n}|\rho_{mn}\rangle\rangle,\end{aligned} \tag{S18}$$

as a super-position of coherent states $|\rho_{mn}\rangle\rangle$ with $c_{m,n}$ being real coefficients that are projections of the $|\rho_{mn}\rangle\rangle$ on the initial density matrix. For $m = n = 0$ DTC density matrix becomes the FSS density matrix and the system does not exhibit any time-crystalline behavior. Otherwise the system exhibits an interference with frequency $|\mathbf{h}|$ between the FSS with frequency scale $\omega$, and coherent oscillations with frequency scale $\lambda$ $(= |\mathbf{h}|\ [\mathrm{mod}\ \omega])$ generated by FDS. Clearly, $|\rho_{DTC}\rangle\rangle$ is not an exact eigen-state of $\hat{\mathcal{U}}_F$ for finite $\gamma$, viz.,

$$\hat{\mathcal{U}}_F|\rho_{DTC}\rangle\rangle = |\rho_{FSS}\rangle\rangle + \sum_{\substack{m,n\\ m,n\neq=0}} c_{m,n}e^{i(m-n)|\mathbf{h}|T}e^{-(m+n)\gamma T}|\rho_{m,n}\rangle\rangle. \tag{S19}$$

The eigenvalues of $\hat{\mathcal{U}}_F$ exhibits two categories, viz., (i) purely real FSS eigenvalue $\mathcal{E}_{FSS}$ corresponding to the value of '1', (ii) coherent state eigenvalues of the form $e^{i\theta_\alpha-(m+n)\gamma T}$, incorporating the decay coming from the FDS-breaking environment. We identify the coherent state eigenvalues as the DTC eigenvalues $\mathcal{E}_{DTC}$ because these are the ones that directly provide the time-period of the underlying time-crystallinity. The FSS eigenvalue can be obtained by projecting $|\rho_{DTC}\rangle\rangle$ on $|\rho_{FSS}\rangle\rangle$ after one period of evolution, viz., $\langle\langle\rho_{FSS}|\hat{\mathcal{U}}_F|\rho_{DTC}\rangle\rangle = 1$, due to the orthogonality condition $\langle\langle\rho_{FSS}|\rho_{coh}\rangle\rangle = 0$. Similarly, the eigenvalues of the coherent states can be found from $\langle\langle\rho_{coh}|\hat{\mathcal{U}}_F|\rho_{DTC}\rangle\rangle$, or in the normal operator notation $\mathrm{Tr}[\rho^{L}_{mn}\mathcal{U}_F\rho^{R}_{mn}]$ where $\rho^{L(R)}_{mn}$ are the left(right) density matrix corresponding to the

coherent states. We notice that for larger integer values of $m, n$, $\hat{\mathcal{U}}_F|\rho_{m,n}\rangle\rangle$ decays much faster. Therefore, it is trivial that the least decaying coherence can only contribute to a DTC density matrix.

Moreover, from (S19) we can recognize that $(m-n)\frac{|\mathbf{h}|[\text{mod }\omega]}{\omega} = q/p$ with $p(>2) \in \mathbb{Z}$ (i.e., integers) & $q/p \in \mathbb{Q}$ (i.e., rational fractions) determines the DTC time-period. When $q/p \notin \mathbb{Q}$ (i.e., irrational fractions) for fractional values of $p$ we find DTQC. In both the cases however, $m-n=q$ will always remain integer valued. Now we proceed on our formulation assuming $p \in \mathbb{Z}$ but our formulation remains valid for fractional $p$ as well. We can write down one such density matrix (out of many possible combinations) as,

$$|\rho_{DTC}\rangle\rangle = |\rho_{FSS}\rangle\rangle + c_{1,0}(|\rho_{1,0}\rangle\rangle + |\rho_{0,1}\rangle\rangle) + c_{2,1}(|\rho_{2,1}\rangle\rangle + |\rho_{1,2}\rangle\rangle), \tag{S20}$$

corresponding to $q=1$ which corresponds to $\frac{|\mathbf{h}|[\text{mod }\omega]}{\omega} = 1/3$ leading to a DTC of time-period $3T$. Therefore,

$$\begin{aligned}\mathcal{E}_{DTC} &= \langle\langle\rho_{coh}|\hat{\mathcal{U}}_F|\rho_{DTC}\rangle\rangle \\ &= e^{i|\mathbf{h}|T}2\left(|c_{1,0}|^2 e^{-\gamma T} + |c_{2,1}|^2 e^{-3\gamma T}\right) \\ &\approx e^{i|\mathbf{h}|T}\left(2[|c_{1,0}|^2 + |c_{2,1}|^2] - 2\gamma T[|c_{1,0}|^2 + 3|c_{2,1}|^2]\right),\end{aligned} \tag{S21}$$

where in the last line we have linearized the exponential decay with respect to $\gamma$. With the choice, $c_{1,0} = c_{2,1} = \frac{1}{2}$ we get,

$$\mathcal{E}_{DTC} = e^{i|\mathbf{h}|T}\left(1 - 2\gamma T\right). \tag{S22}$$

Eq. (S22) reproduces what we have obtained numerically in Supplementary Figure 1(b). There can be other combinations corresponding to other integer values of $q$ as well. For example, $|\rho_{DTC}\rangle\rangle = |\rho_{FSS}\rangle\rangle + c_{2,0}(|\rho_{2,0}\rangle\rangle + |\rho_{0,2}\rangle\rangle)$ with $c_{2,0} = \frac{1}{\sqrt{2}}$, corresponding to $q=2$ can also satisfy (S22) with the oscillating part being $e^{2i|\mathbf{h}|T}$ which also corresponds to DTC frequency $\lambda = 2|\mathbf{h}|$ [mod $\omega$]. This density matrix corresponds to $|\mathbf{h}|/\omega = 2/3$ also leading to DTC of time-period $3T$.

Let us now discuss the notion of stability and meta-stability. Looking closely the spectrum of $\mathcal{U}_F$ in Supplementary Figure 2(a) it can be recognized that the FSS lies on the real axis on the unit circle. Then stable coherent states states are those which lie on the unit circle but not on the real axis. The meta-stable DTC states lie near the unit circle (but not on it). Supplementary Figure 2(a) shows that these meta-stable states (the red dots) do not coalesce to the FSS (the red square) but their magnitude decay maintaining the phase (therefore the rigidity of the DTC sub-harmonic frequency), viz., $\mathcal{E}_{DTC}(t) = e^{i|\mathbf{h}|t}e^{-2\gamma t}$, as shown above. Therefore, these states are distinct from the FSS, and form a low lying (meta-stable) manifold.

## SUPPLEMENTARY NOTE 2. WEAK LOCAL FDS AS AN EMERGENT PROPERTY NEAR THE FSS

In deriving (S17) from (S12)-(S13) we have implicitly assumed $\left[\mathcal{H}_0, (S^+_{loc,|\mathbf{h}|}(t)\ )^m\right]$ vanishes. In order to explicitly show that this is indeed the case we consider an example of Floquet coherent state that satisfies the scaling behavior shown in the Supplementary Figure 2(c) of our main text, viz., $\rho_{2,0}(t) = \left[S^+_{loc,|\mathbf{h}|}(t)\right]^2 \rho_{FSS}$. We are interested in the long-time dynamics of the FCS, viz., $\lim_{t\to\infty}\rho_{2,0}(t)$ quite in line with Ref. [10]. Note that the Floquet coherent state (FCS) is built on the FSS and it's equation of motion is given by,

$$\begin{aligned}\frac{d\rho_{2,0}(t)}{dt} &= \frac{d(S^+_{loc,|\mathbf{h}|}(t)\ )^2}{dt}\rho_{FSS}, \\ &= i\left[\mathcal{H}_0, (S^+_{loc,|\mathbf{h}|}(t)\ )^2\right]\rho_{FSS} + 2i(|\mathbf{h}| - \gamma)(S^+_{loc,|\mathbf{h}|}(t)\ )^2\rho_{FSS} \\ &= i\left[\mathcal{H}_0, (S^+_{loc,|\mathbf{h}|}(t)\ )^2\right]\rho_{FSS} + 2i(|\mathbf{h}| - \gamma)\rho_{2,0}(t).\end{aligned} \tag{S23}$$

All we need to show that $i\left[\mathcal{H}_0, (S^+_{loc,|\mathbf{h}|}(t)\ )^2\right]\rho_{FSS}$ vanishes under sufficiently general conditions. First, it can be easily numerically be verified that $i\left[\mathcal{H}_0, (S^+_{loc,|\mathbf{h}|}(t)\ )^2\right]\rho_{FSS}$ vanishes even after a few driving periods. For this go back to the lab frame (L).

We first find FSS from the eigenvalue equation $U_F^{(L)}(T,0)(\rho^{(L)}_{FSS}) = (\rho^{(L)}_{FSS})$ in the Lab frame (denoted by the superscript $(\cdot)^{(L)}$). The $\rho^{(L)}_{FSS}$ corresponds to the red-dot in Supplementary Figure 2(a) of the main text. Then in the Lab-frame we time evolve the well known ad-joint master equation (S7) corresponding to $(S^+_{loc,|\mathbf{h}|}(t)\ )^2$ for duration

of $t = 2T$ for $\gamma = \omega$ (corresponding to very large dissipation) and $t = 20T$ for $\gamma = 10^{-5}\omega$ (corresponding to very small dissipation). Note that this should ideally be for a long duration but we find that the above duration already establish our results. Then a direct computation of $i\left[\mathcal{H}_0, (S^+_{loc,|\mathbf{h}|}(t)\ )^2\right]\rho^{(L)}_{FSS}$, shows that it vanishes.

Therefore, (S23) becomes $\frac{d\rho_{2,0}(t)}{dt} = 2i(|\mathbf{h}|-\gamma)\rho_{2,0}(t)$. The solution of this equation is $\rho_{2,0}(t) = e^{2i(|\mathbf{h}|-\gamma)(t-t')}\rho_{2,0}(t')$. The time evolution for a duration equal to the driving period $T$ then leads to,

$$\rho_{2,0}(t'+T) = U_F(T,0)(\rho_{2,0}(t')\ ) = e^{2i(|\mathbf{h}|-\gamma)T}\rho_{2,0}(t'), \tag{S24}$$

which proves our proposition of weak local FDS. To this end we conclude that weak local FDS does not appear as an exact operator relationship, rather it emerges from the Floquet steady state.

## SUPPLEMENTARY NOTE 3. NOTION OF WEAK-FLOQUET DYNAMICAL SYMMETRY

In Ref. [9], the strong dynamical symmetry (DS) corresponds to a conserved quantity $S$ with respect to both Hamiltonian and Liouvillian evolution, viz., $[S,H]=0$, $[S,V_\mu]=[S,V_\mu^\dagger]=0$. A weak dynamical symmetry condition, $\mathcal{L}(S\rho S^\dagger) = (S\mathcal{L}[\rho]S^\dagger)$, where $\hat{\mathcal{L}}$ is a super-operator, equation A.2, comes from the fact that although $[S,V_\mu]=[S,V_\mu^\dagger]\neq 0$ for individual $\mu$, $[S,H]=0$, and $\mathcal{D}[S\rho S^\dagger]=0$. This leads to the condition $[\hat{\mathcal{L}},\hat{S}]=0$ in the super-operator notation, equation A.7 which comes from the fact that $\mathcal{L}[S\rho S^\dagger] = S\rho(t)S^\dagger$ at all time $t$ and for all the solutions of $\frac{d\rho}{dt}=\mathcal{L}[\rho]$. Note that $S$ needs to be a symmetry operator of the Hamiltonian for all these relationships to be satisfied.

The strong dynamical symmetry condition has been extend to incorporate the condition when $S$ become an eigen-operator instead of a symmetry operator [10, 11]. In this case, the strong dynamical symmetry corresponds to an operator $S$ satisfying $[S,H]\rho_{SS} = -\lambda S\rho_{SS}$, $[S,V_\mu]\rho_{SS} = [S,V_\mu^\dagger]\rho_{SS} = 0$ [10, 11]. The Liouvillian then exhibits purely imaginary eigenvalues, viz., $\hat{\mathcal{L}}|\rho\rangle\rangle = i\lambda|\rho\rangle\rangle$, leading to the appearance of DTC via dynamical symmetry mechanism. Since $S$ in no longer a symmetry operator, for any density matrix of the form $|\rho\rangle\rangle = \hat{S}|\rho_{SS}\rangle\rangle$ where $\hat{\mathcal{L}}|\rho_{SS}\rangle\rangle = 0$, it has been shown $[\hat{\mathcal{L}},\hat{S}]|\rho_{SS}\rangle\rangle = i\lambda\hat{S}|\rho_{SS}\rangle\rangle$, i.e., $\hat{S}$ is an eigen-operator of the Liouvillian super-operator (a strong dynamical symmetry implies the weak one).

In our case, we find a local operator $[S_{loc}, V_{1(N)}] = [S_{loc}, V^\dagger_{1(N)}] \neq 0$, which importantly leads to $\mathcal{D}[S_{loc}\rho S^\dagger_{loc}] = -\gamma S_{loc}$. This leads to an eigen-value condition $[\hat{\mathcal{L}},\hat{S}_{loc}]|\rho_{SS}\rangle\rangle = (i\lambda-\gamma)\hat{S}_{loc}|\rho_{SS}\rangle\rangle$. In the case of Floquet system we have just replaced $\hat{\mathcal{L}}$ with the Floquet-map $\hat{\mathcal{U}}_F$ at the necessary places and the eigen-value will be replaced by $(e^{(i\lambda-\gamma)T}-1)$.

Therefore, our condition corresponds to an eigen-value condition similar to the strong dynamical symmetry, viz., $[\hat{\mathcal{L}},\hat{S}_{loc}]|\rho_{SS}\rangle\rangle = (i\lambda-\gamma)\hat{S}_{loc}|\rho_{SS}\rangle\rangle$, together with $[S_{loc}, V_{1(N)}] = [S_{loc}, V^\dagger_{1(N)}] \neq 0$. This led us to choose the terminology of weak-local dynamical symmetry in the main text. The I blow summarizes various notions related to the dynamical symmetry (DS):

| strong DS in Ref. [9] | weak DS in Ref. [9] | strong DS in Ref. [10, 11] | weak DS in the manuscript |
|---|---|---|---|
| $[S,H]=0$, and<br>$[S,V_\mu]=[S,V_\mu^\dagger]=0$ | $[S,H]=0$, and<br>$[S,V_\mu]=[S,V_\mu^\dagger]\neq 0$<br>$\mathcal{D}[S\rho S^\dagger]=0$ leading $[\hat{\mathcal{L}},\hat{S}]=0$ | $[H,S]=\lambda S$<br>$[S,V_\mu]=[S,V_\mu^\dagger]=0$<br>$[\hat{\mathcal{L}},\hat{S}]|\rho_{SS}\rangle\rangle = i\lambda\hat{S}|\rho_{SS}\rangle\rangle$ | $[H,S_{loc}]=\lambda S_{loc}$<br>$[S_{loc},V_{1(N)}]=[S_{loc},V^\dagger_{1(N)}]\neq 0$<br>$[\hat{\mathcal{L}},\hat{S}_{loc}]|\rho_{SS}\rangle\rangle = (i\lambda-\gamma)\hat{S}_{loc}|\rho_{SS}\rangle\rangle$ |

**Supplementary Table** I. Summary of notion of weak and strong dynamical symmetry available in the literature.

## SUPPLEMENTARY NOTE 4. SYSTEM SIZE N=5

We further consider a 5-site system to show that the conclusions obtained for a 3-site system remains the same. This is representative of a large system; 5-site system is a mid-way between what can be realized in semiconductor QD experiments (usually between 3 or 4 coupled dots have been realized, see Ref. [12]) and in optical-lattices (usually very large lattice size [13]). To demonstrate we consider DTC corresponding to $B=\frac{4\pi}{3}$ MHz with dephasing strength $\Gamma = 0.1t_{hop}$. Note that we have chosen $t_{hop}=\omega$ however, the results are independent of the specific choice of parameters. Supplementary Figure 1 shows synchronized oscillation of $\langle S^y_j(t)\rangle$ with period $3T$ for all the 5-sites with the same oscillation profile as seen for the 3-site system, see Figure 4 of the main text for a comparison. Therefore,

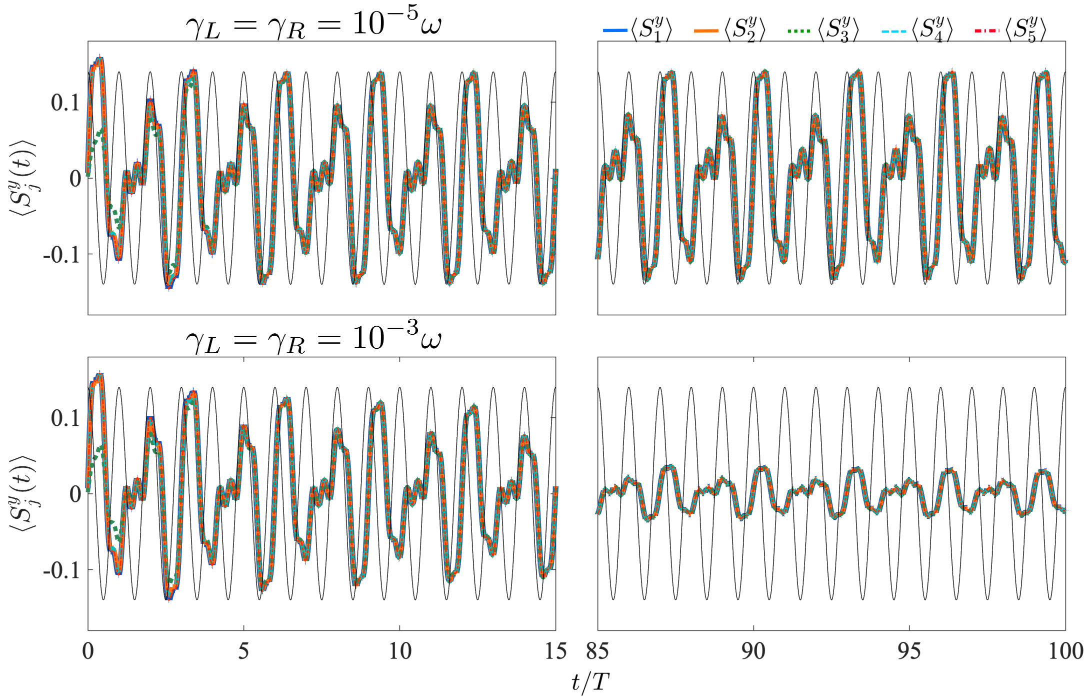


**Supplementary Figure** 1. Plots of the time evolution of $\langle S_j^y(t)\rangle$ ($j = 1-5$) corresponding to stable DTC [system-lead coupling $\gamma = 10^{-5}\omega$] and meta-stabel DTC [system-lead coupling $\gamma = 10^{-3}\omega$] as a function of the dimensionless time $t/T$. Black line represents $\cos(\frac{2\pi t}{T})$, the driving period.

we conclude that all the conclusions obtained from the 3-site system remain true for 5-site system, and based on our analytical formulation described in Sec. SUPPLEMENTARY NOTE 1 should remain true for infinite system as well.

## SUPPLEMENTARY NOTE 5. DEPHASING RATE DEPENDENCE OF SUB-HARMONIC SYNCHRONIZATION

In quantum regime two subsystems, say $S_1$ and $S_2$, initialized into independent configurations, are said to be in complete "quantum-synchronization" if they acquire identical trajectories under the effects of mutual interactions [14]. In the context of our system the above definition translates to the following. If oscillation of any/all of spin-component corresponding to each site of the Fermi-Hubbard chain is locked to the same frequency and phase, and exhibits the same magnitude independent of the specific value of any microscopic parameters then we say that each site has achieved a complete "quantum-synchronization." In terms of the limit cycles, each site then exhibits the exact same limit cycle, therefore, the exact same phase space trajectory.

Supplementary Figure 2 shows how the dephasing affects the synchronization defined above. To probe synchronization we plot $\langle S_j^y(t)\rangle$ ($j = 1, 2, 3$) for three different values of dephasing rate $\Gamma = (0.1t_{hop},\ 10^{-3}t_{hop},\ 10^{-6}t_{hop})$ for stable DTC [Supplementary Figure 2(a)] and meta-stable DTC [Supplementary Figure 2(b)]. For both cases we find that for very weak dephasing corresponding to $\Gamma = 10^{-6}t_{hop}$ [bottom panel of Supplementary Figure 2(a) and (b)], although the first and the last sites are completely synchronized in terms of both oscillation frequency and magnitude, the middle site is not. The middle site exhibits the same frequency as the other sites but the magnitude of oscillation is different. The reason for the first and the last sites being completely synchronized is that these are connected to the external leads with the exact same value of the system-lead coupling, whereas, middle site experiences only the dephasing. With an increased dephasing rate corresponding to $\Gamma = 10^{-3}t_{hop}$ we see, from the middle panel of Figs. 2(a) and (b), that the magnitude of spin-oscillation corresponding to the middle site starts to decay and ultimately matches with the other two sites in the long time limit on a time scale $\Gamma^{-1}$ [not shown]. For even stronger dephasing rate corresponding to $\Gamma = 0.1t_{hop}$ we see, from the top panel of Figs. 2(a) and (b) all the three sites are completely synchronized within 10 driving periods ($\sim \Gamma^{-1}$).

We conclude that due to the exact same system-lead coupling the first and the last sites are always synchronized no matter what the value of the dephasing rate is. All the sites that are not connected to the leads develop a time scale

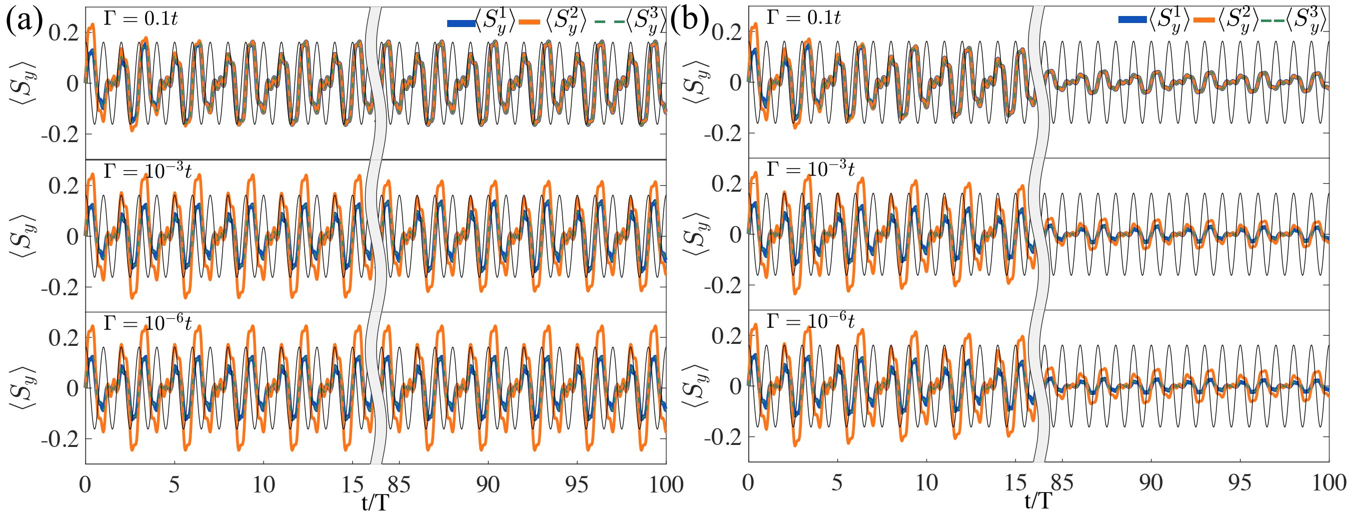


**Supplementary Figure** 2. (a) Plots of the time evolution of $\langle S_j^y(t)\rangle$ ($j=1,2,3$) corresponding to stable DTC [system-lead coupling $\gamma = 10^{-5}\omega$] as a function of the dimensionless time $t/T$ in the long-time limit for three values of dephasing rates $\Gamma = 0.1t_{hop}$ (top panel), $\Gamma = 10^{-3}t_{hop}$ (middle panel), and $\Gamma = 10^{-6}t_{hop}$ (bottom panel). (b) Plots of the time evolution of $\langle S_j^y\rangle$ ($j=1,2,3$) corresponding to meta-stable DTC [system-lead coupling $\gamma = 10^{-3}\omega$] as a function of the dimensionless time $t/T$ in the long-time limit for three values of dephasing rates $\Gamma = 0.1t_{hop}$ (top panel), $\Gamma = 10^{-3}t_{hop}$ (middle panel), and $\Gamma = 10^{-6}t_{hop}$ (bottom panel). Black line represents $\cos(\frac{2\pi t}{T})$, the driving period.

$\sim \Gamma^{-1}$, determined by the dephasing rate, that is required by them to get completely synchronized with the sites at both ends of the array.

In order to demonstrate the above conclusions are true independent of the system size, we further show that for 4-site and 5-site systems dephasing strength still brings in the synchronization. Supplementary Figure 3 plots the $\langle S_j^y(t)\rangle$ as a function of dimensionless time ($t/T$) for both 4-site (lower panel) and 5-site (upper panel) systems. It shows that the sites connected to the leads (boundary sites) always remain synchronized due to the system-lead coupling of the exact same strength acting on these sites. The other sites grows with time which eventually gets synchronized with boundary sites on a time-scale $\Gamma^{-1}(\approx 50T)$.

## SUPPLEMENTARY NOTE 6. SPIN-CURRENT

At the steady state the system satisfies charge-current continuity equation, viz., $\frac{dQ}{dt} = \hat{J}$, where $J = \sum_\sigma(\hat{J}_{L,\sigma} + \hat{J}_{R,\sigma})$ is the total current through the system. Since the system is connected to external magnetic field there is no charge accumulation which leads to conservation of the total charge. The equation of motion for the total charge density operator $Q = en = \sum_{j,\sigma} en_{j,\sigma}$ is evaluated from (S7),

$$e\sum_{j,\sigma}\frac{dn_{j,\sigma}}{dt} = ie\left[\mathcal{H}(t), \sum_{j,\sigma} n_{j,\sigma}\right] + \sum_\sigma(\hat{J}_{L,\sigma} + \hat{J}_{R,\sigma}) = \sum_\sigma(\hat{J}_{L,\sigma} + \hat{J}_{R,\sigma}), \tag{S25}$$

where $\hat{J}_{L,\sigma} = e\gamma_L(1 - n_{1,\sigma})$ is the current corresponding to spin $\sigma$ going into the system from the left lead, and $\hat{J}_{R,\sigma} = e\gamma_R n_{N,\sigma}$ is the current corresponding to spin $\sigma$ going out of the system from the right lead, with $e$ being the electronic charge. In our calculation we expressed all the energy and time scales in the units of $MHz$, therefore $e\gamma_{L(R)}$ directly gives Ampere. Then the spin current through the right lead is defined as $\hat{J}_s = e\gamma_R(n_{N,\uparrow} - n_{N,\downarrow})$, used in Eq. (3) of the main text.

[1] A. Riera-Campeny, M. Moreno-Cardoner, and A. Sanpera, Time crystallinity in open quantum systems, Quantum **4**, 270 (2020).

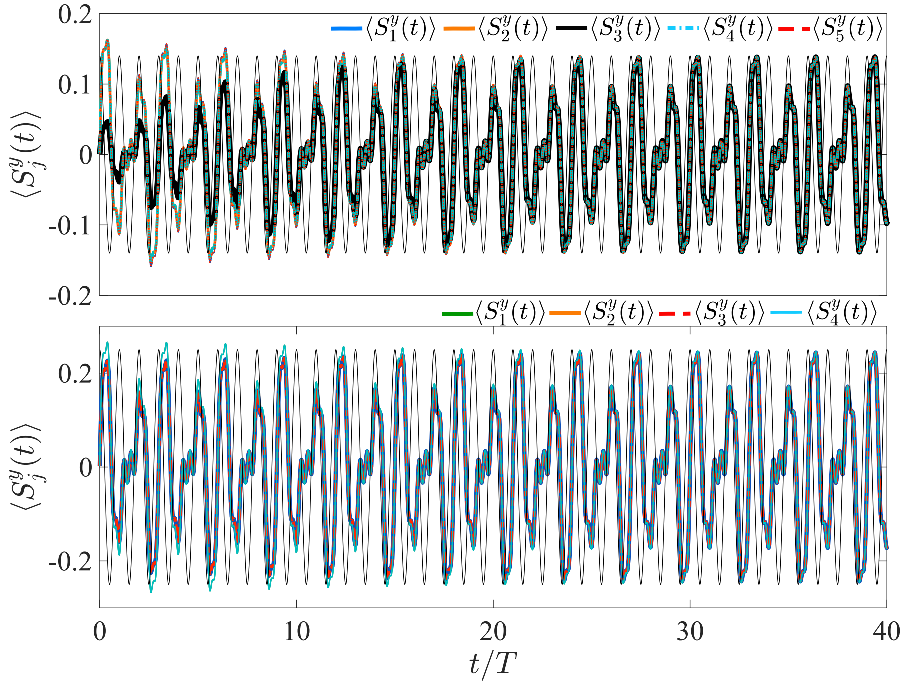


**Supplementary Figure** 3. Plots of the time evolution of $\langle S_j^y(t)\rangle$ corresponding to stable DTC [system-lead coupling $\gamma = 10^{-5}\omega$] as a function of the dimensionless time $t/T$ for the dephasing strength $\Gamma = (1/50)t_{hop}$. Upper and lower panels correspond to 5-site and 4-site systems, respectively. Black line represents $\cos(\frac{2\pi t}{T})$, the driving period. 1.


[2] T.-S. Ho, K. Wang, and S.-I. Chu, Floquet-liouville supermatrix approach: Time development of density-matrix operator and multiphoton resonance fluorescence spectra in intense laser fields, Phys. Rev. A **33**, 1798 (1986).

[3] T. Prosen and E. Ilievski, Nonequilibrium phase transition in a periodically driven $xy$ spin chain, Phys. Rev. Lett. **107**, 060403 (2011).

[4] D. Vorberg, W. Wustmann, R. Ketzmerick, and A. Eckardt, Generalized bose-einstein condensation into multiple states in driven-dissipative systems, Phys. Rev. Lett. **111**, 240405 (2013).

[5] M. Hartmann, D. Poletti, M. Ivanchenko, S. Denisov, and P. Hänggi, Asymptotic floquet states of open quantum systems: the role of interaction, New Journal of Physics **19**, 083011 (2017).

[6] K. Chinzei and T. N. Ikeda, Time crystals protected by floquet dynamical symmetry in hubbard models, Phys. Rev. Lett. **125**, 060601 (2020).

[7] D. Manzano, A short introduction to the lindblad master equation, AIP Advances **10**, 025106 (2020), https://doi.org/10.1063/1.5115323.

[8] J. H. Shirley, Solution of the schrödinger equation with a hamiltonian periodic in time, Phys. Rev. **138**, B979 (1965).

[9] B. Buča and T. Prosen, A note on symmetry reductions of the lindblad equation: transport in constrained open spin chains, New Journal of Physics **14**, 073007 (2012).

[10] B. Buča, J. Tindall, and D. Jaksch, Non-stationary coherent quantum many-body dynamics through dissipation, Nature Communications **10**, 1730 (2019).

[11] J. Tindall, C. S. Muñoz, B. Buča, and D. Jaksch, Quantum synchronisation enabled by dynamical symmetries and dissipation, New Journal of Physics **22**, 013026 (2020).

[12] T. Hensgens, T. Fujita, L. Janssen, X. Li, C. J. Van Diepen, C. Reichl, W. Wegscheider, S. Das Sarma, and L. M. K. Vandersypen, Quantum simulation of a fermi–hubbard model using a semiconductor quantum dot array, Nature **548**, 70 (2017).

[13] C. Gross and I. Bloch, Quantum simulations with ultracold atoms in optical lattices, Science **357**, 995 (2017), https://science.sciencemag.org/content/357/6355/995.full.pdf.

[14] A. Mari, A. Farace, N. Didier, V. Giovannetti, and R. Fazio, Measures of quantum synchronization in continuous variable systems, Phys. Rev. Lett. **111**, 103605 (2013).
